# Supplementary material for: GraCIAS: Grassmannian of Corrupted Images for Adversarial Security
Source: arXiv:2005.02936 source file (2020-05-07)
Supplement: Supplementary file 1 [file additional.tex]

\section{Applications}
% GraCIAS has achieved state-of-the-art results across different models on ImageNet dataset across different attacker strength. With this success, we also see the potential of it being used as a data augmentation technique in network training. Additionally, it can also be used as an image processing tool prior to processing with simpler defense to boost their performance. 
\begin{wraptable}{r}{0.6\textwidth}
     \centering
     \begin{tabular}{c|ccc}
     \hline
        Datasets & ImageNet & ImageNet & CIFAR10\\
         Model & InceptionV3 & ResNet50 & ResNet \\\hline
         Original & 78 & 76&94.6 \\
          With Defense &62.8 &53.4 & 55.5\\\hline 
     \end{tabular}
     \caption{Classification Accuracy on Clean Samples with \textbf{GraCIAS} defense. The drop is expected on clean samples as the network has not seen such transformation during network training}
     \label{tab:clean}
 \end{wraptable}{}
\begin{figure}{r}[h]
    \centering
    \includegraphics[width= 0.45\textwidth]{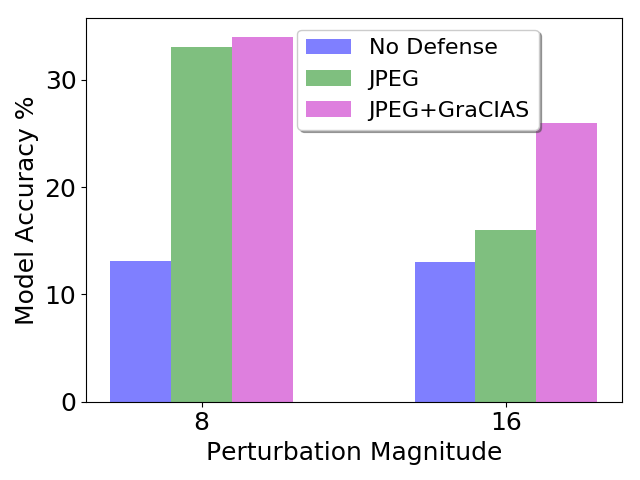}
    \caption{CIFAR10 Dataset: Performance of JPEG vs JPEG+GraCIAS as defense for different values of  $\epsilon$. The merit of combining with GraCIAS is more evident for larger adversarial perturbation.}
    % (Right) Defense Accuracy under BPDA for varying magnitude of $\epsilon$. Std. Model is the original model and  'GraCIAS trained' is the model trained with GraCIAS transformation as data augmentation for training. }
    \label{fig:cifar_bpda}
\end{figure}

% \begin{wraptable}{r}{0.6\textwidth}
%      \centering
%      \begin{tabular}{c|ccc}
%      \hline
%         Datasets & ImageNet & ImageNet & CIFAR10\\
%          Model & InceptionV3 & ResNet50 & ResNet \\\hline
%          Original & 78 & 76&94.6 \\
%           With Defense &62.8 &53.4 & 55.5\\\hline 
%      \end{tabular}
%      \caption{Classification Accuracy on Clean Samples with \textbf{GraCIAS} defense. The drop is expected on clean samples as the network has not seen such transformation during network training}
%      \label{tab:clean}
%  \end{wraptable}{}
%  \vspace{-0.4cm}
